# Supplementary material for: Fixed points of Wegner-Wilson flows and many-body localization
Source: arXiv:1607.07884 ancillary file (2016-07-26)
Supplement: Supplementary file 1 [file sup.pdf]

# Supplement: Fixed points of Wegner-Wilson flows and many-body localization

David Pekker,<sup>1,2</sup> Bryan K. Clark,<sup>3</sup> Vadim Oganesyan,<sup>4,5</sup> and Gil Refael<sup>6</sup>

<sup>1</sup>*Department of Physics and Astronomy, University of Pittsburgh, Pittsburgh, PA 15260, USA*

<sup>2</sup>*Pittsburgh Quantum Institute, Pittsburgh, PA 15260, USA*

<sup>3</sup>*Department of Physics, University of Illinois at Urbana Champaign, IL 61801, USA*

<sup>4</sup>*Department of Engineering Science and Physics,*

*College of Staten Island, CUNY, Staten Island, NY 10314, USA*

<sup>5</sup>*Physics program, The Graduate Center, CUNY, New York, NY 10016, USA*

<sup>6</sup>*Department of Physics and the Institute for Quantum Information and Matter, Caltech, Pasadena, CA 91125, USA*

## I. COMPRESSING THE STRUCTURE OF $H(\beta)$ AND $U(\beta)$

How does the complexity of  $H(\beta)$  and  $U(\beta)$  depend on the WWF flow parameter  $\beta$  and how much can these matrices be collapsed? In order to quantitatively address these questions we ran WWF flow on a ten site chain with various amounts of disorder. At each step of the flow we converted the  $H(\beta)$  and  $U(\beta)$  into a matrix product operator representation using the standard machinery (keeping singular vectors with  $\lambda > 0.0001$ ). We plot the bond dimensions of the resulting operators, as a function of  $\beta$ , for various disorder strengths in Fig. 1. We observe that the bond-dimension of  $U(\beta)$  increases mainly monotonically with the flow, while the bond dimension of  $H(\beta)$  first increases, as new multi-site couplings are generated, and then decreases as the Hamiltonian is brought to diagonal form. Moreover, the bond dimensions throughout the flow are bounded by the bond dimension of  $U(\beta \rightarrow \infty)$ . We point out that this observation, in combination with numerical evidence that in the fully-MBL systems  $U(\beta \rightarrow \infty)$  can be compactly represented [1], implies that in the fully-MBL systems  $H(\beta)$  and  $U(\beta)$  can be compactly represented for the entire duration of the WWF.

[1] D. Pekker, B.K. Clark, arXiv:1410.2224.

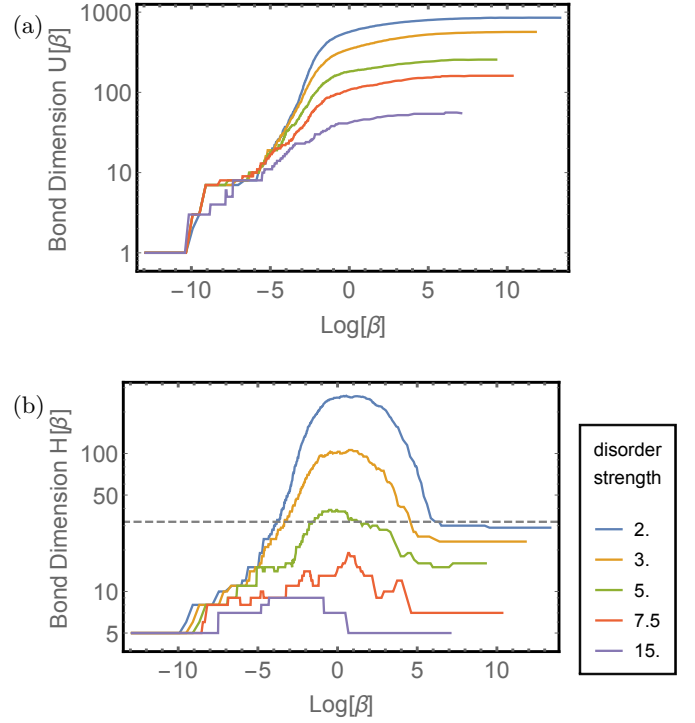

FIG. 1. Bond dimension of the MPO representation of  $U(\beta)$  (a) and  $H(\beta)$  as a function of  $\beta$  for several disorder strengths (legend). The calculation was performed on a length 10 chain. The dashed line in (b) indicates the maximal bond dimension for diagonal Hamiltonians with  $L = 10$ ; it is essentially saturated for the case disorder strength  $w = 2$ .

## II. ALTERNATE VISUALIZATIONS OF THE DISTRIBUTIONS OF $|J_{ijk...}|$

In Fig. 1 of the main text we presented a selection of the full distribution functions of the couplings  $|J_{ijk...}|$  of the diagonal Hamiltonian.

We begin by re-plotting these distribution using “logarithmic” variables  $\zeta = \log(|J|/\text{median}[|J|])$  (see Fig. 2). This method of plotting provides a complimentary method for the visualization of the narrowing of the distributions in the ergodic phase and the widening of the distributions in the MBL phase.

Next, we present a “waterfall plot” of the full distribution functions for all disorder strengths  $w$  and all ranges  $4 \leq r \leq 12$  (see Fig. 3). Just as in Fig. 1 of the main text, for each  $w$  and  $r$  we normalize the  $J$ 's by their median to make comparison of the distributions at different ranges possible. We observe that the distributions plotted in Fig. 3 smoothly morph from broad and  $1/\mathcal{J}$ -like at the top of the figure to narrow and flat at the bottom of the figure. To make this smooth morphing apparent we ordered the distributions, not by  $w$  nor  $r$ , but instead by the small  $J$  power law (Fig. 4 of the main text). In the MBL phase, this ordering tends to put *large*  $r$ 's and *large*  $w$ 's towards the top of Figure. Similarly, in the ergodic phase this ordering tends to put *large*  $r$ 's and *small*  $w$ 's towards the bottom of Figure. At intermediate disorder  $w \sim 4$ , the distributions are largely  $r$  independent and hence are clumped by  $w$ . The smooth morphing of the distributions implies that there is a one parameter family of distributions

$$\mathcal{F}_{w,r}(\tilde{J}) = \mathcal{F}_{f(r,w)}(\tilde{J}), \quad (1)$$

where  $\tilde{J} = |J|/\text{median}[|J|]$  and  $f(r,w)$  is a real valued function.

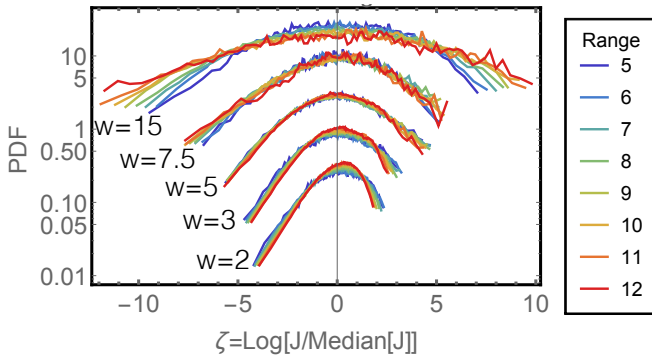

FIG. 2. Distributions of the logarithmic variable  $\zeta$ . Distributions at different disorder strengths have been shifted vertically for clarity.

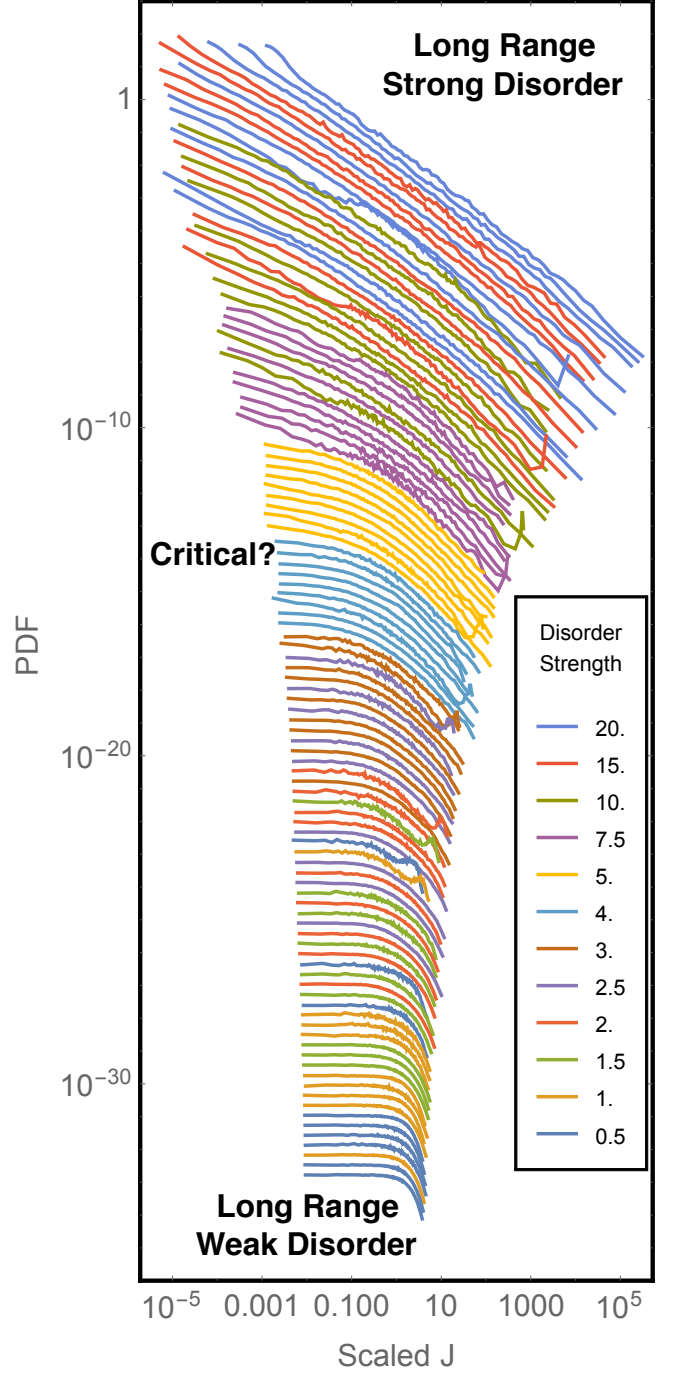

FIG. 3. Distribution  $\mathcal{F}_{w,r}(\tilde{J})$  of  $|J_{i,j,...,k}|$ 's the  $\ell$ -bit couplings in the end-point Hamiltonians of Wegner flow across a wide range of disorder strength spanning the MBL-to-ergodic phase transition. We characterize the distributions  $\mathcal{F}_{w,r}(\tilde{J})$  by two parameters: (1) the disorder strength  $w$  and (2) the range  $r$ . To make comparison of distributions at different disorder strengths and ranges possible, we scale the distributions so that their median is unity. The distributions are ordered by the power law for small  $J$ 's and each subsequent distribution is shifted down slightly for clarity. The range  $r$  is a proxy for a coarse graining parameter. We observe that for critical disorder strength,  $w \sim 4$ , the distributions are independent of  $r$ , while away from criticality the distributions are  $r$ -dependent.

### III. FILTERING BY OPERATOR NUMBER

In the main text we discussed how the distribution of the couplings  $J_{ijk\dots}$  depends on range  $r$  and disorder strength  $w$ . Let us define  $m$  to be the number of  $\tau^z$ 's, i.e.  $J_{1,5}$  corresponds to  $m = 2$ , while  $J_{1,3,5}$  corresponds to  $m = 3$ . Does the distribution of couplings  $J_{ijk\dots}$  depend on  $m$ ? Surprisingly we find that for our model Hamiltonian it does not.

We begin by plotting  $\text{Median}[|J|]$  as a function of  $m$  at fixed  $r$  and  $w$  (see Fig. 4). We observe that at large ranges  $r = 12$  (yellow lines with open diamonds) there is essentially no dependence on  $m$ , except for the limiting cases  $m = 2$  and  $m = 12$ . Next, we dig deeper and look at the distributions of  $J_{ijk\dots}$  (see Fig. 6). Again, we find that except for the limiting cases,  $m = 2$  (dashed lines) and  $m = r$  (gray lines), at fixed  $w$  and  $r$  there is essentially no dependence of the distribution on  $m$ .

We conclude this section by remarking about this result from the perspective of perturbation theory. Consider the free version of the Hamiltonian

$$H_0 = \frac{1}{4}t_{xy} \sum_i [\sigma_i^x \sigma_{i+1}^x + \sigma_i^y \sigma_{i+1}^y] + \frac{1}{2} \sum_i h_i \sigma_i^z, \quad (2)$$

we should find that the diagonal Hamiltonian must be of the Anderson form

$$H_{\text{diag}} = \frac{1}{2} \sum_i J_i \tau_i^z, \quad (3)$$

which is indeed the form obtained by running WWF. Let us now add the perturbation Hamiltonian

$$H_1 = \frac{1}{4}t_z \sum_i \sigma_i^z \sigma_{i+1}^z. \quad (4)$$

For small values of  $t_z$  one expects to be able to construct a perturbation theory and hence find  $J_{ijk\dots} \sim (t_z/t_{xy})^{m-1}$ . As we move to the Heisenberg model regime  $t_z/t_{xy} = 1$ , this perturbation theory evidently breaks down and the dependence on  $m$  disappears.

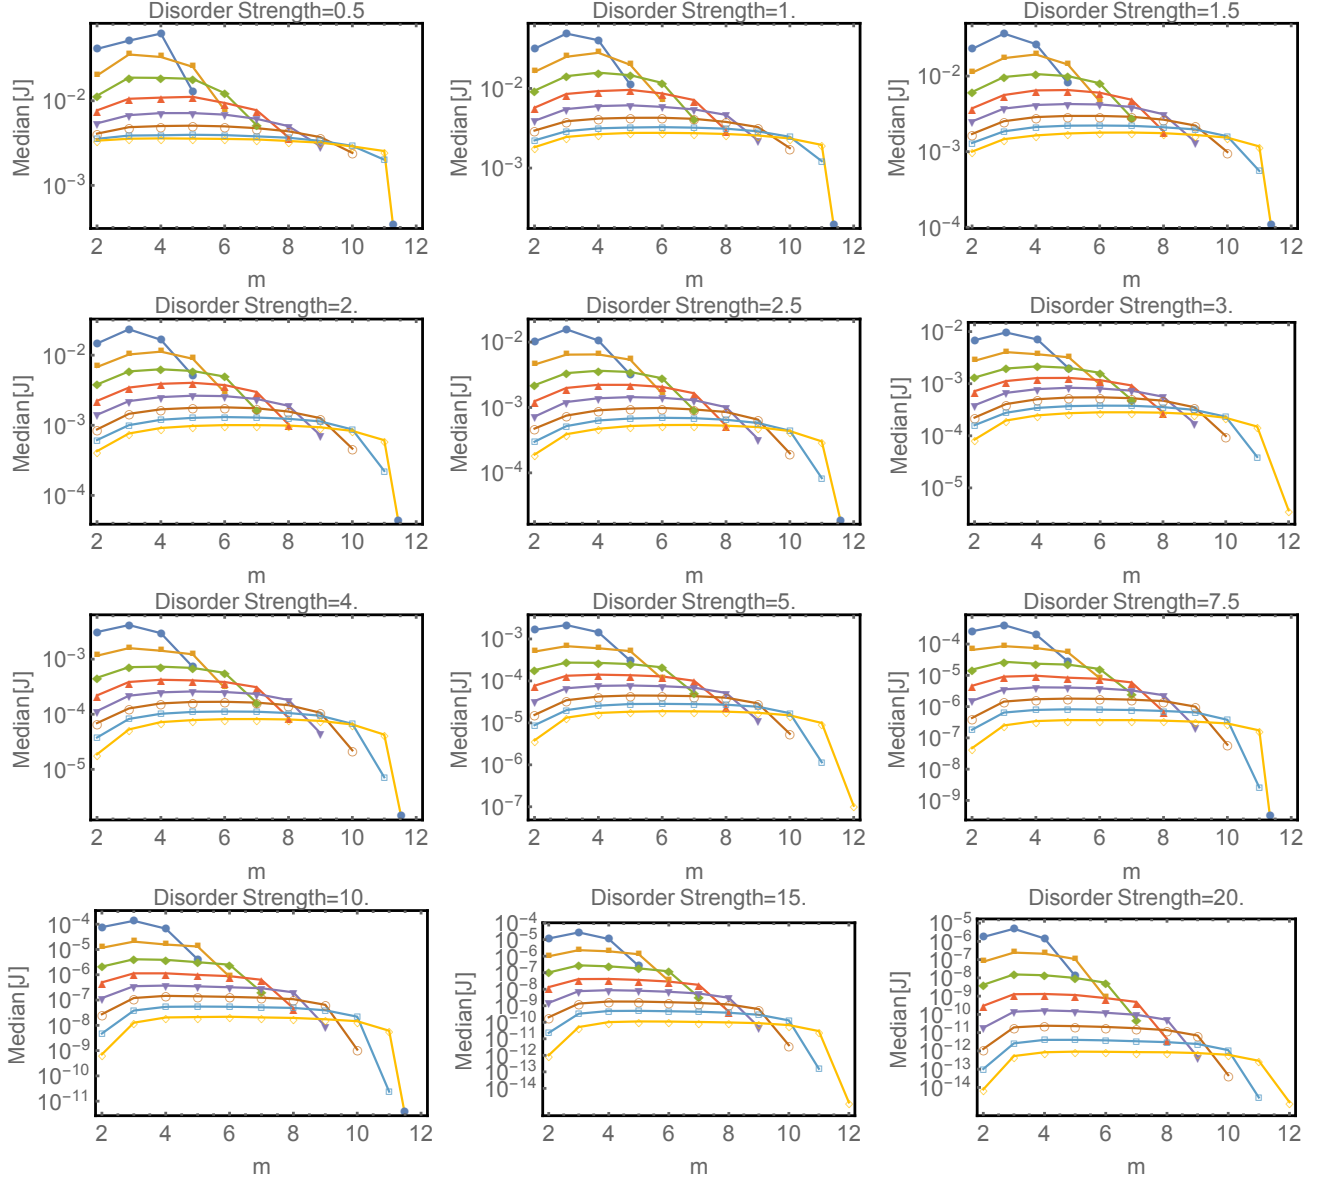

FIG. 4. Median[ $|J|$ ] as a function of the number of operators in the interaction term  $m$  for various ranges  $r$  (different colored lines) and disorder strengths  $w$  (different panels). The colors of the curves represent different ranges, from  $r = 5$  (top blue) to  $r = 12$  (bottom yellow).

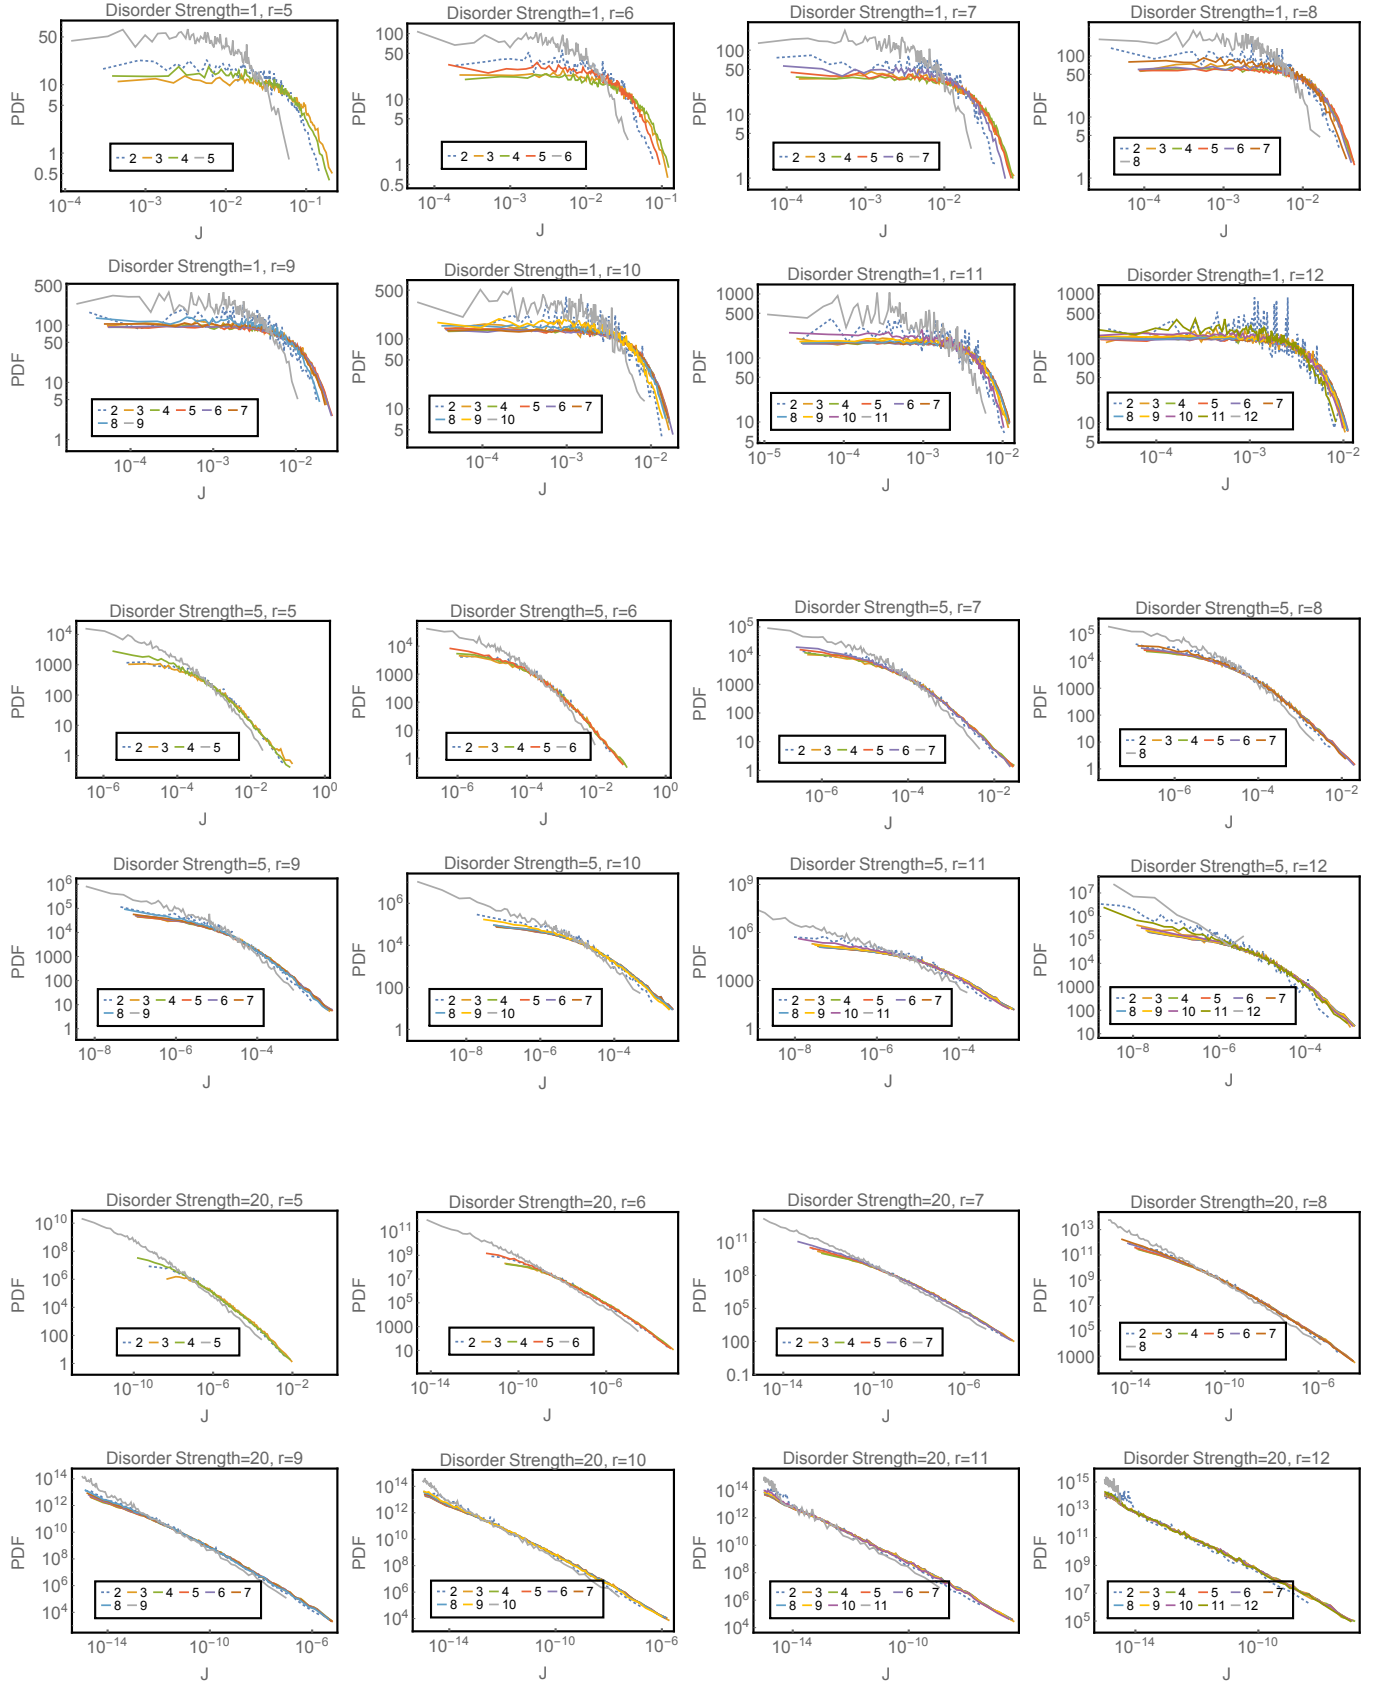

FIG. 5. Distribution of  $J$ 's at fixed disorder strength  $w$  and range  $r$  (different panels) as a function of operator number  $m$  (different colored lines, see legend in each panel). Observe that within each panel all distributions (with the exception of  $m = 2$  and  $m = r$ ) look essentially identical.

#### IV. DISTRIBUTION OF EFFECTIVE TWO SPIN INTERACTIONS

In this appendix we compare the distributions of couplings that appears in the diagonal Hamiltonian to distributions of effective two-site couplings  $C_{ij}[\vec{a}]$ . Consider the four eigenstates  $|a_1, \dots, a_{i-1}, \alpha \dots a_{j-1}, \beta \dots a_L\rangle$  (in the l-bit basis) which differ on sites  $i$  and  $j$  but are equal to the bits  $\vec{a}$  on all other sites. We define  $C_{i,j}[\vec{a}] = \frac{1}{4}(E_{\uparrow\uparrow} + E_{\downarrow\downarrow} - E_{\uparrow\downarrow} - E_{\downarrow\uparrow})$ . The distributions are over both the frozen l-bits in  $\vec{a}$  as well as the pair  $(i, j)$  which sets the range. The two ways of representing l-bits interactions are linearly related, albeit with a non-trivial transform. Note that, well inside the ergodic and MBL phases  $W = 0.5$  and  $W = 15$ , respectively, we observe very similar behaviors.

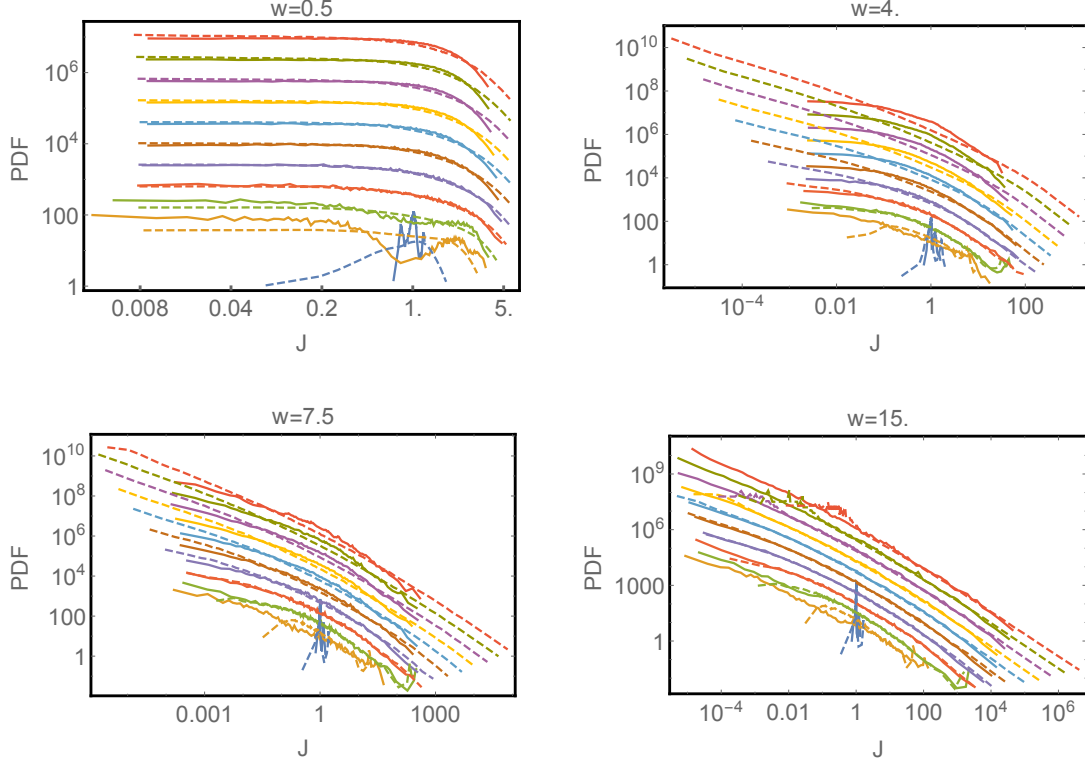

FIG. 6. The horizontal axis is labelled by coupling strength normalized by the median for that disorder and range. Solid lines are reproductions from Fig. 1 of distributions of l-bit couplings. Dashed lines are distributions of effective two l-bit couplings.
